# Supplementary material for: Quantum superresolution in fluorescence microscopy
Source: arXiv:1212.6003 source file (2013-07-11)
Supplement: Supplementary file 1 [file Supplementary.pdf]

# Supporting information for
# Quantum superresolution in fluorescence microscopy

O. Schwartz,[1] J.M. Levitt,[1] R. Tenne,[1] S. Itzhakov,[1] Z. Deutsch,[1] and D. Oron[1]
[1] *Department of Physics of Complex Systems, Weizmann Institute of Science, Rehovot, Israel*

## QUANTUM DOTS

Quantum emitters used in this work were CdSe/CdS/ZnS colloidal quantum dots with the main emission peak at 617 nm. The QDs were synthesized as follows: a mixture of cadmium oxide (CdO), n-tetradecylphosphonic acid (TDPA), and 1-octadecene (ODE) was heated under argon to 280°C in a three-neck flask. The stock solution of trioctylphosphine selenium (TOPSe) was quickly injected to the hot solution. The growth temperature was then reduced to 250°C until the dots reached the desired diameter. The CdS and ZnS shells were synthesized using a layer-by-layer growth technique in a one-pot synthesis [1].

The quantum yield of these QDs was measured to be 0.62 at 530 nm excitation. The absorption and emission spectra of the QDs are shown in Fig. SI1.

The samples used for superresolution imaging were prepared by dispersing QDs in toluene solution of Poly(methyl methacrylate), which was then spin-coated onto glass slides.

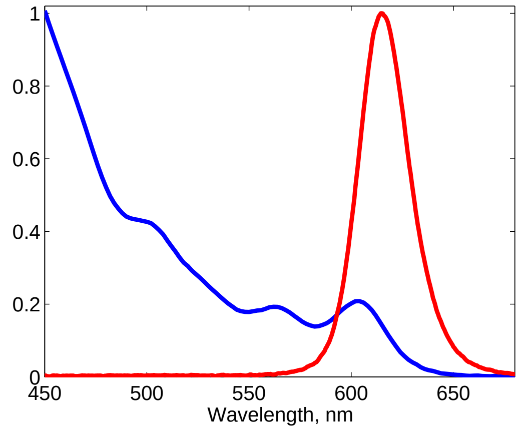


Fig. SI1. QD absorption spectrum (blue) and their emission spectrum (red), in arbitrary units.

## EXPERIMENTAL SETUP

The EMCCD (Andor iXon3) was operating at the maximal gain, in the 'cropped sensor' mode. Limiting the field of view to 98 by 62 pixels allowed us to perform data acquisition at 997.1 Hz, which was within 0.1 Hz of the laser repetition rate. The camera was not actively triggered by the laser, but was running free synchronously with it. The camera was operated in the frame transfer mode, meaning that the CCD was exposed and the optical signal was collected during the entire 1.003 ms interval between frames. The actual optical signal, QD fluorescence, reached the camera within few tens of nanoseconds after the laser pulse, and for the rest of the exposure time, only spurious photons leaking from the environment were detected. Since the laser repetition rate was close to the EMCCD frame rate, there was one laser pulse per frame in most frames, the probability of two or zero pulses occurring in the same exposure cycle being less than $10^{-4}$. For excitation, we used the second harmonic of a Q-switched Nd:YAG laser from Teem Photonics with a pulse duration of 300 ps. Quantum dots exhibit antibunching due to Auger interactions, which lead to very fast non-radiative decay of multi-excitons. On the other hand, the pulse duration is considerably shorter than the QD fluorescence lifetime of 32 ns, so multiple photon emission following a single pulse was strongly suppressed[2]. The pulse energy was chosen so as to excite the QDs at or around the saturation threshold [2].

## DATA PROCESSING

Superresolution information is contained in both intensity auto-correlations in the image plane and in cross-correlations between independent adjacent detectors (pixels)[3]. In this work, we focus on cross-correlations between adjacent pixels in the CCD, since cross- correlations can be readily observed in the photon counting regime. In every frame, the raw EMCCD readings were thresholded to produce a map of photon detection events. The probability for two photons to be detected in the same pixel within one excitation cycle was kept low, and we neglect it in our data processing.

Classically the readings in the two detectors would be uncorrelated:

$$\left\langle N_1^{\rm cl} N_2^{\rm cl} \right\rangle = \left\langle N_1^{\rm cl} \right\rangle \left\langle N_2^{\rm cl} \right\rangle . \quad (1)$$

If the emission is antibunched, the photon can hit only one of any two detectors, leading to measurable correlations between them. In the second order, the antibunching signal can be defined as cross-correlation:

$$A^{(2)} = \langle N_1 N_2 \rangle - \langle N_1 \rangle \langle N_2 \rangle, \quad (2)$$

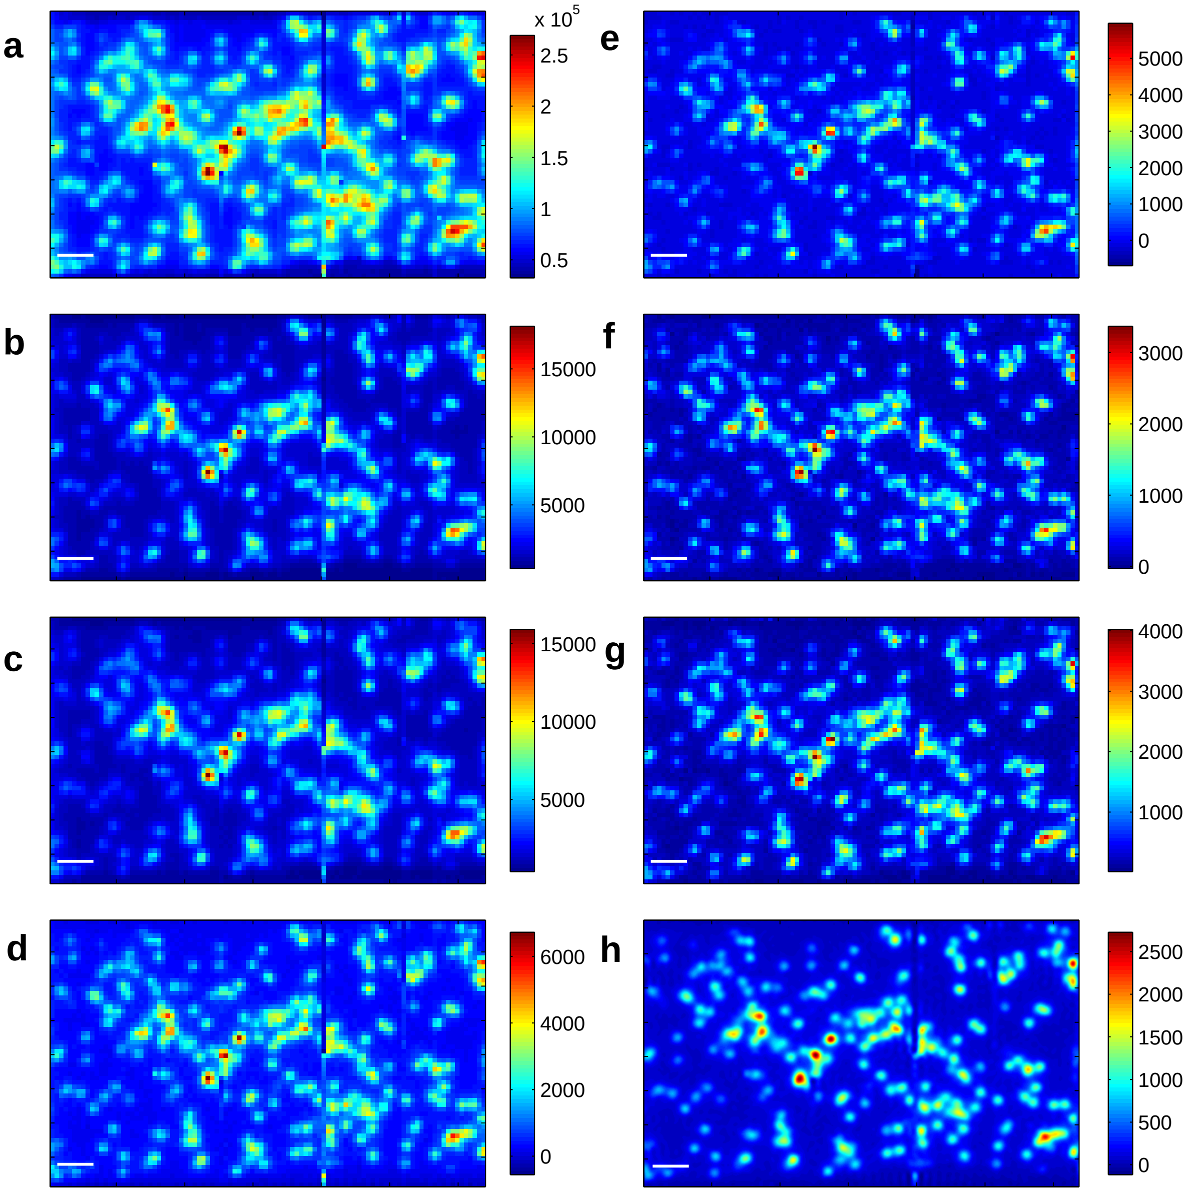


Fig. SI2. **Intermediate images illustrating the data processing for second order antibunching imaging.** **a**, map of photon detection events obtained by thresholding raw CCD data. **b**, map of two photon coincidence events for one of the two-pixel configurations, the horizontal nearest neighbors. **c**, the 'correlation baseline' appearing as the correction term in eq.4. Panel **d** shows the second order antibunching signal for the horizontal pair pixel configuration, given by a linear combination of panels **b** and **c**. Panels **e-g** show the second order antibunching signal for the three remaining pixel pair configurations. The last panel shows the superresolved antibunching image, obtained by combination of the four previous images. Scalebar length is $1\mu m$. The vertical line visible in all the images at about $x = 8\mu$m is due to a 'hot' pixel in the CCD.

where $N_{1,2}$ are the numbers of photons detected in the first and second detector following exposure to a single excitation pulse. The angle brackets denote quantum mechanical expectation values, which are experimentally evaluated by averaging the relevant quantities over our datasets. The antibunching signal is computed for the four pixel pair configurations shown in Fig.1(b). This yields four images, with each data point corresponding to a given pixel pair. The data points are thus associated with the antibunching signal sampled in the geometrical center of that pair, which falls either on a pixel side (for horizontal and vertical pairs) or in a vortex point between four pixels (diagonal pairs). The four antibunching images were Fourier interpolated and spatially filtered to obtain a smooth correlation map. The high resolution image was then produced as the sum of the four component images.

The image filtering above was performed by applying

a coefficient of $\frac{ka}{2}/\sin(\frac{ka}{2})$, where $a$ is the pixel size, to the Fourier component with the spatial frequency $k$. The coefficient is close to unity at low spatial frequencies and approaches the maximal value of $\pi/2$ at the highest spatial frequency. This filter removes the blurring caused by pixelation, assuming that the pixel pitch allows for above-Nyquist sampling. This filter was used throughout this work for all the second and third order antibunching component images, as well as for the regular fluorescence images.

The third order signal was produced by detecting correlations in the three-pixel configurations shown in Fig. 1(c). The third order antibunching signal should be an additive statistical quantity, describing the nonclassical third order correlations between three detectors, while excluding the pairwise correlations already taken into account in the second order. The relevant statistic is given by the irreducible part of the third order correlation function, also known as the connected correlation function or cross-cumulant:

$$A^{(3)} = \langle N_1 N_2 N_3 \rangle + 2\langle N_1\rangle\langle N_2\rangle\langle N_3\rangle - \Big(\langle N_1 N_2\rangle\langle N_3\rangle + \langle N_2 N_3\rangle\langle N_1\rangle + \langle N_3 N_1\rangle\langle N_2\rangle\Big) \quad (3)$$

This signal quantifies the missing triple coincidence events, excluding the ones that are induced by the missing photon pairs, already accounted for in the second order. Once the signal has been computed for the four three-pixel configurations, the images were interpolated and combined similarly to the second order.

**Camera artefact treatment**

In practice, the pixel readings in an EMCCD are not uncorrelated even when detecting classical light. Fig. 1(e) illustrates the typical cross-correlation between two adjacent pixels. The sharp peak in the center indicates the presence of the shot to shot fluctuations in the detection process, which make the detection events appear bunched even when in reality they are not. This, in addition to longer-term fluctuations due to imperfect temperature stabilization, clock voltage drifts, etc, requires a modification of our data treatment. In the second order signal processing, we account for the spurious correlations as follows. The measured cross-correlation at small non-zero delays is used to estimate the apparent bunching peak in the cross-correlation, assuming no photon correlations. The signal is then given by the difference between that estimate and the actual cross-correlation at zero delay.

The second order antibunching signal is thus estimated using the following expression:

$$A^{(2)} = \big\langle N_1(i)N_2(i)\big\rangle_i - R\frac{1}{10}\sum_{k=-5..5,k\neq 0}\big\langle N_1(i)N_2(i+k)\big\rangle_i, \quad (4)$$

where $N_{1,2}(i)$ denotes the number of photons detected in the corresponding pixel in frame $i$, the angle brackets denote averaging over $i$, and the coefficient $R$ serves to correct for the apparent bunching of the EMCCD readings. The coefficient is chosen separately for each of the four types of pixel pairs shown in Fig.1(b), but is kept constant for the entire image series.

In the third order, the signal is estimated in a similar manner, although more coefficients must be used to account for apparent bunching.

$$A^{(3)} = \Big\langle N_1(i)N_2(i)N_3(i)\Big\rangle_i + 2\,\frac{1}{10}H\sum_{p,\,q}\Big\langle N_1(i)N_2(i+p)N_3(i+q)\Big\rangle_i - \\ -\frac{1}{10}\,S\sum_k\Big\langle N_1(i+k)N_2(i)N_3(i) + N_1(i)N_2(i+k)N_3(i) + N_1(i)N_2(i)N_3(i+k)\Big\rangle_i, \quad (5)$$

where the index $k = -5...5$, $k \neq 0$, and $p$ and $q$ assume the following ten values: $(p, q) = (1, -2)$, $(1, -1)$, $(1, 2)$, $(2, -1)$, $(2, 1)$, $(-1, -2)$, $(-1, 1)$, $(-1, 2)$, $(-2, -1)$, $(-2, 1)$. The correction coefficients $S$ and $H$ were chosen empirically to cancel the apparent bunching of the classical signal. In the antibunching signal (5), the first term is the three-point correlation at zero delay, the second, with the correction coefficient, provides the 'uncorrelated photons' baseline, and the last term is necessary to account for the contribution of the second order correlations.

**Data processing examples**

In this section we give an example of the intermediate steps in building the antibunching images.

Fig. SI2 illustrates the process of generating a second order antibunching image. Panel (a) shows an image

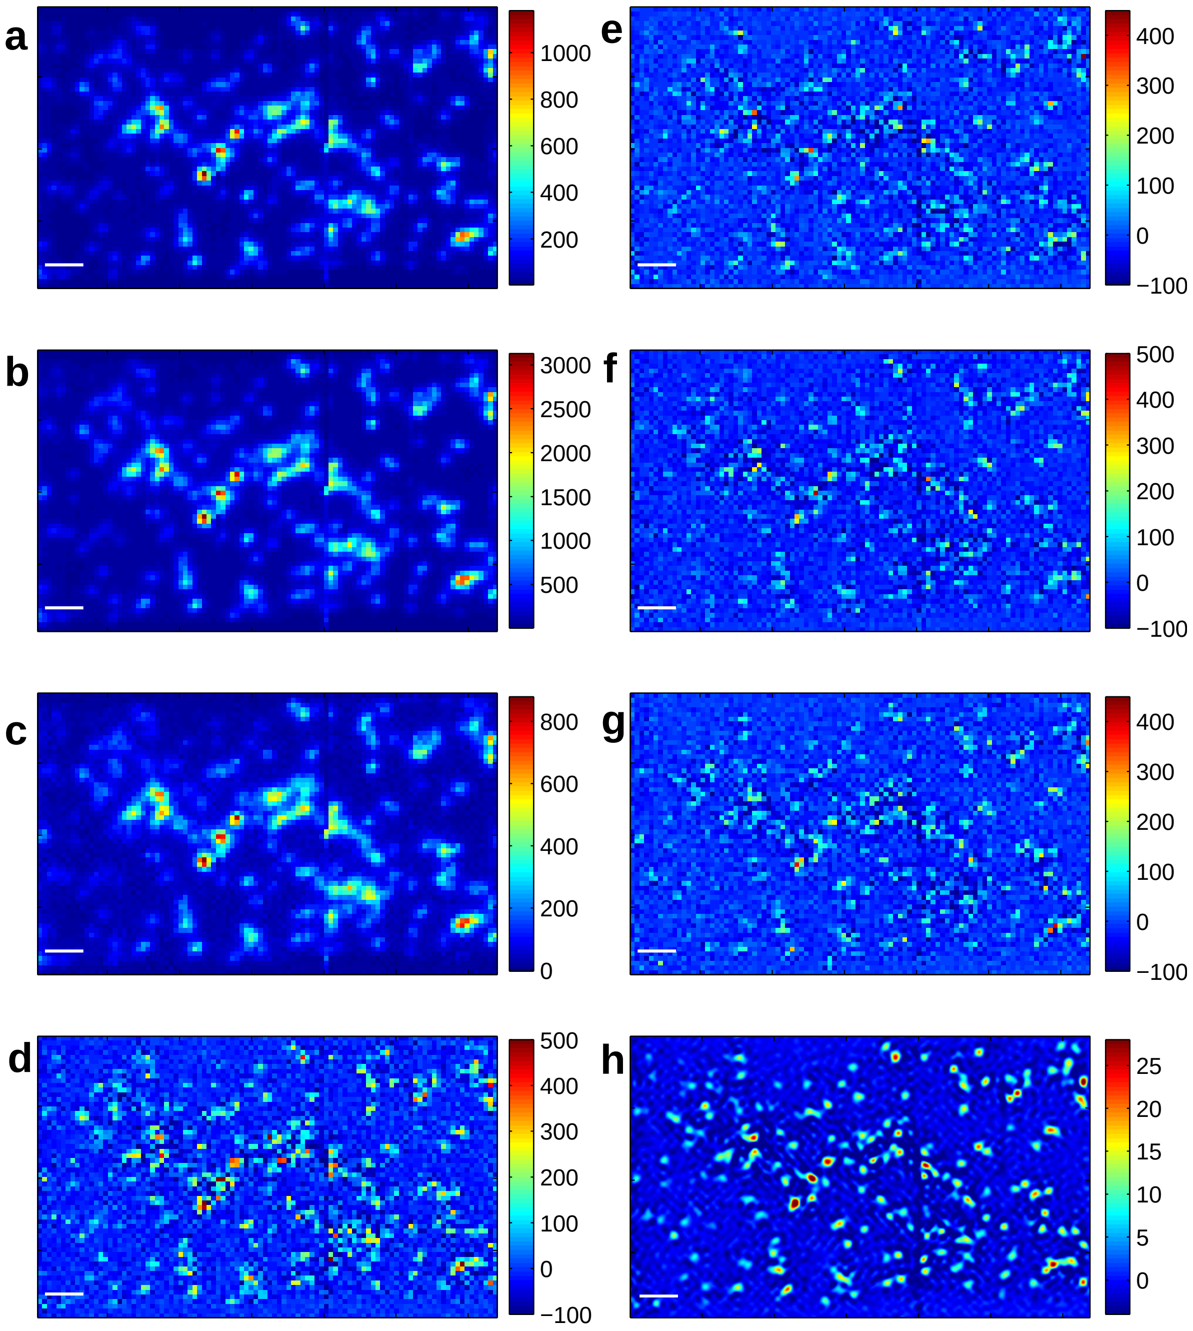


Fig. SI3. **Third order antibunching data processing**. Panels **a-c** demonstrate the three terms of eq.5 for a given three-pixel configuration. Panel **d** shows the third order antibunching signal given by a linear combination of panels **a-c**. The antibunching signals for the remaining three-pixel configurations are shown in panels **e-g**. The images are combined, similarly to the second order, to produce the superresolved third order antibunching image shown in the last panel. Scalebar, $1\mu m$.

obtained by thresholding a series of 4 million images. Fig. SI2(b) shows a map of two-photon coincidence events for two pixels forming a horizontal pair. Fig. SI2(c) demonstrates the correlation 'baseline', representing the second term in eq. (4). Fig. SI2(d) shows the difference between the images of Fig. SI2(b) and Fig. SI2(c), corresponding to the antibunching signal of (4) for a horizontal pair. Panels Fig. SI2(e-g) show the antibunching signal for the three remaining types of pixel pair shown in Fig.1(b) The four images of Fig. SI2(d-g) are interpolated, and the resulting oversampled images are shifted to align the pixel pair centers in the same coordinate sys-

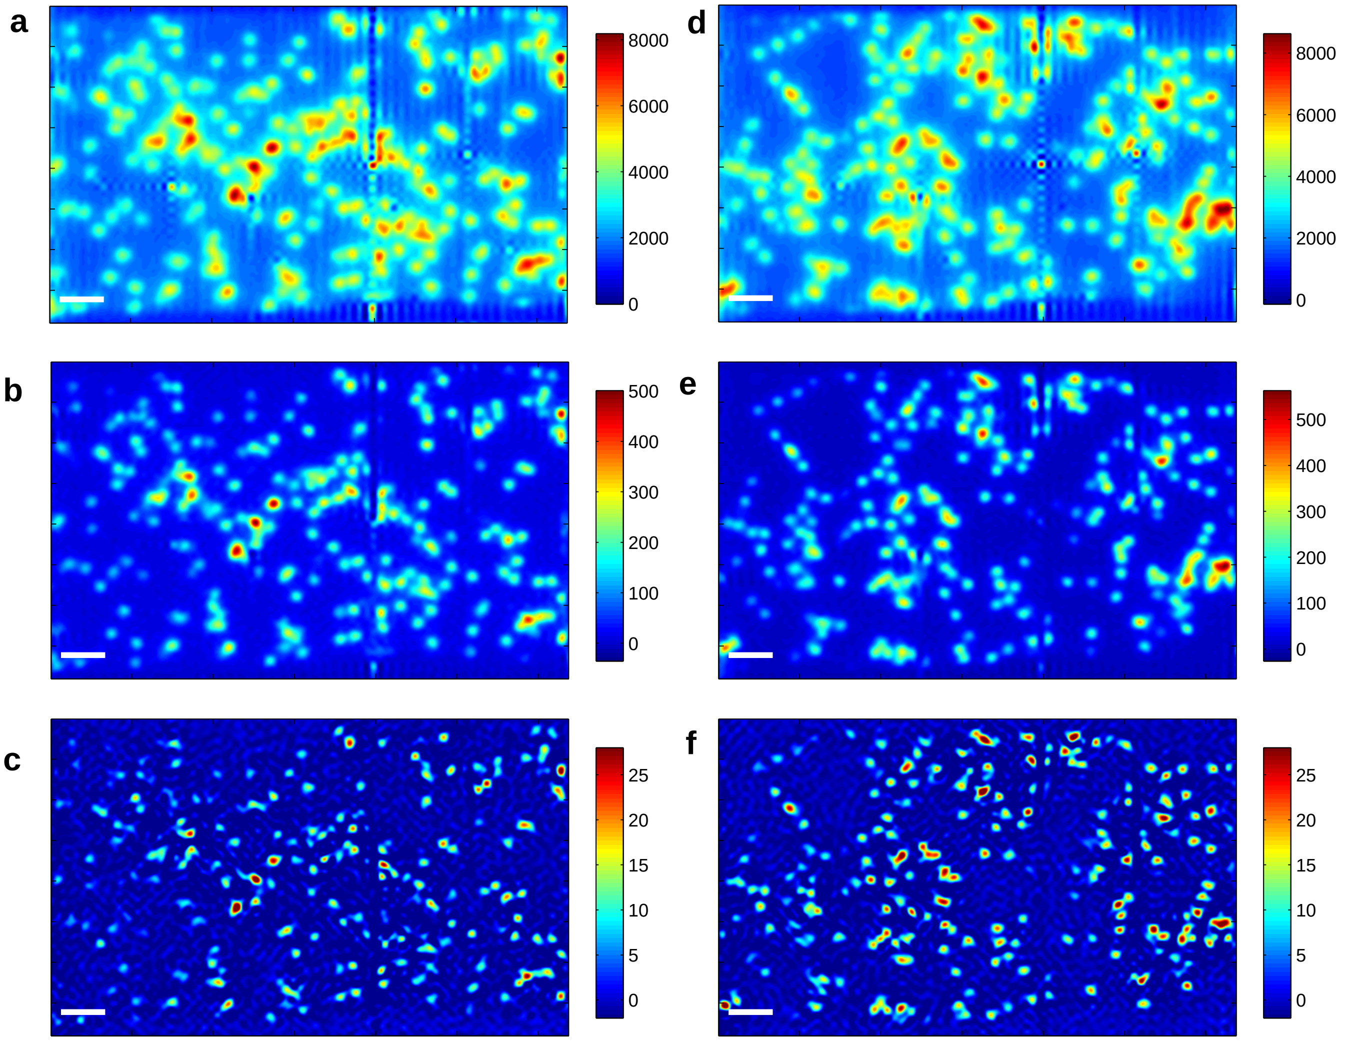


Fig. SI4. **Two sets of antibunching images**. **a,d**: regular fluorescence. **b,e**: second order antibunching images. **c,f**: third order antibunching images. The colormap is saturated to highlight the resolution enhancement. Both image sets correspond to 1.1 hours of integration (4 million frames). Scalebar is $1\mu m$.

tem. The four images are then summed to produce the superresolved image shown in Fig. SI2 (h).

The third order data processing is illustrated in Fig. 3. Fig. SI3(a) shows a map of three-photon coincidence events detected for one of the three-pixel configurations shown in Fig. 1c. The next two panels, Fig. SI3 (b) and (c), show the two subtraction terms of eq.(5) for the same pixel configuration. The antibunching signal of eq.(5), representing a linear combination of Fig. SI3 (a-c), is shown in Fig. SI3(d). Panels Fig. SI3(e-g) show similar antibunching signals for other three-pixel configurations. The four images are combined, similarly to the 2nd order, to produce the third order superresolution image shown in Fig. SI3(h).

Two examples of second and third order antibunching images are given in Fig. SI4. The two upper panels (Fig. SI4 a,d) show regular fluorescence images obtained by interpolating the thresholded EMCCD data. The middle panels (Fig. SI4 b,e) show the corresponding second order antibunching images, demonstrating a clear improvement of resolution. The bottom two panels (Fig. SI4 c,f) show the third order antibunching images with further enhanced resolution. Both image sets are produced from a set of 4 million one-exposure CCD frames (1.1 hour of integration).

## RESOLUTION QUANTIFICATION

Although improved resolution is evident in the antibunching images above, it is important to provide a quantitative measure of the resolution enhancement.

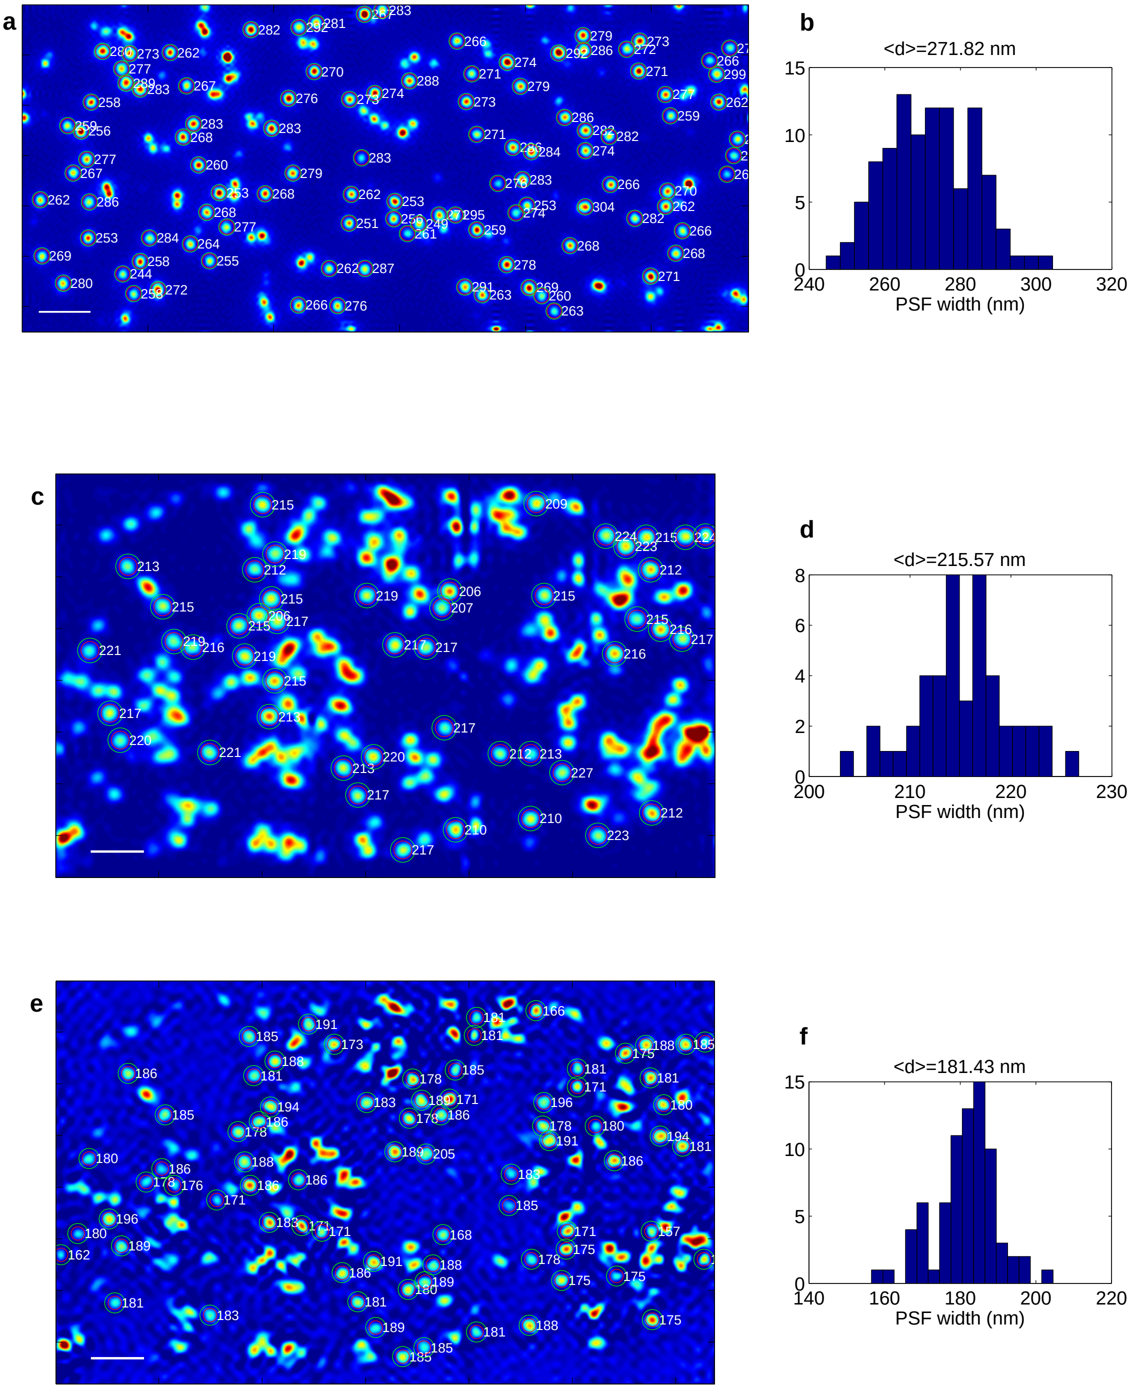


Fig. SI 5. **Resolution quantification.** **a**, an image with a number of isolated QDs used for resolution estimation. A histogram of the FWHM diameters of the QD images is shown in **b**. Panels **c, d** show a 2nd order antibunching image and the corresponding diameter distribution. Panels **e,f** show the same for a third order antibunching image. In panel **a**, scalebar is $2\mu m$, in panels **c** and **e**, $1\mu m$.

The resolution enhancement in antibunching imaging was assessed by measuring full width at half maximum (FWHM) of the effective point spread function. Due to the significant level of noise present in the antibunching images, we took a statistical approach to resolution quantification. For an ensemble of well separated individual quantum dots visible in an antibunching image, the FWHM was determined as follows. For every quantum dot, the maximum signal, corresponding to the brightest pixel in its image, was determined. The background level was estimated as the mean signal in a ring of inner diameter 500 nm and outer diameter of 700 nm, centered on the brightest pixel. The middle between the maximum and the background was set as the half-maximum level. The number of pixels with the signal above half maximum was counted and used to determine the area above the half maximum. The FWHM was then calculated as the diameter of a circle with the same area.

In this manner, the image width was computed for a number of quantum dots, shown in Fig. SI5(a). A histogram of the resulting FWHM distribution is shown in Fig. SI5(b). Based on the mean of the distribution shown, the PSF FWHM of the regular fluorescence imaging in our system is 272 nm.

Although a naive application of the frequently used paraxial approximation formula, $d_o = \lambda/2NA \simeq 220$nm, where $NA = 1.4$ stands for the microscope objective numerical aperture, gives a much smaller PSF width, this approximation is not valid for high numerical aperture microscopy. When calculating the expected PSF width theoretically, one should consider that for high resolution microscope objectives the effective numerical aperture is usually somewhat lower than the nominal due to apodization and high-order aberrations at the edge of the objective aperture [4, 5]. In addition, the resolution is significantly decreased by vectorial effects, which elongate the PSF in the polarization direction for linearly polarized light and cause PSF broadening for unpolarized[6]. Taking these factors into account, our figure agrees well with the literature[7–9].

The same PSF width estimation method applied to the antibunching images gave 216 nm for the second order (see Fig. SI5 (c,d)) and 181 nm (Fig. SI5 (e,f)) for the third order. These results correspond to a resolution increase by a factor of 1.26 in the second order and a factor of 1.5 in the third order.

These numbers are lower than the theoretically expected resolution enhancement factors of $\sqrt{2} \simeq 1.41$ and $\sqrt{3} \simeq 1.73$ for the second and third order, respectively. A major factor contributing to this discrepancy is the finite pixel size. Experimentally, a tradeoff exists between the signal to noise level, which improves when pixels are larger, and the resolution, which is limited by the pixel size. We chose the magnification of the microscope to have an effective pixel size of $d = 130$ nm, which would provide Nyquist-limited sampling at a spatial frequency corresponding to an effective wavelength of $\lambda_N = 2d = 260$nm. This is a factor of 1.7 shorter than the wavelength corresponding to the shortest transverse spatial frequency accessible in our microscope $\lambda_m = \lambda/NA = 440$nm. Thus our sampling frequency is sufficient for imaging with resolution enhancement up to a factor of 1.7. On the other hand, the finite pixel size limits us to detecting the nonclassical intensity correlations between points separated by a considerable fraction of the PSF width, which may cause a certain resolution deterioration compared to the idealized experiment wherein correlations are probed in adjacent points.


[1] J.J. Li, Y.A. Wang, W. Guo, J.C. Keay, T.D. Mishima, M.B. Johnson, and X. Peng. Large-scale synthesis of nearly monodisperse cdse/cds core/shell nanocrystals using air-stable reagents via successive ion layer adsorption and reaction. *Journal of the American Chemical Society*, 125(41):12567–12575, 2003.

[2] O. Schwartz, R. Tenne, J.M. Levitt, Z. Deutsch, S. Itzhakov, and D. Oron. Colloidal quantum dots as saturable fluorophores. *ACS nano*, 2012.

[3] O. Schwartz and D. Oron. Improved resolution in fluorescence microscopy using quantum correlations. *Physical Review A*, 85(3):33812, 2012.

[4] R. Juškaitis. Measuring the real point spread function of high numerical aperture microscope objective lenses. *Handbook of biological confocal microscopy*, pages 239–250, 2006.

[5] Stefan W Hell, Pekka E Hänninen, Ari Kuusisto, Martin Schrader, and Erkki Soini. Annular aperture two-photon excitation microscopy. *Optics communications*, 117(1):20–24, 1995.

[6] M. Gu. *Advanced optical imaging theory*, volume 75. Springer, 1999.

[7] T. Wilson, R. Juškaitis, and P. Higdon. The imaging of dielectric point scatterers in conventional and confocal polarisation microscopes. *Optics communications*, 141(5):298–313, 1997.

[8] R. Juškaitis and T. Wilson. The measurement of the amplitude point spread function of microscope objective lenses. *J. Microsc*, 189(1):8–11, 1998.

[9] A. Marian, F. Charrière, T. Colomb, F. Montfort, J. Kühn, P. Marquet, and C. Depeursinge. On the complex three-dimensional amplitude point spread function of lenses and microscope objectives: theoretical aspects, simulations and measurements by digital holography. *Journal of Microscopy*, 225(2):156–169, 2007.
